# Supplementary material for: Mesh Total Generalized Variation for Denoising
Source: arXiv:2101.02322 source file (2021-06-08)
Supplement: Supplementary file 1 [file appendix.tex]

\newpage
\section*{Appendix}
\begin{lemma} \label{lemma1}
The adjoint operator of $\overline{\mathcal{D}}_{\mathcal{E}}$, that is $\overline{\mathcal{D}}^{\star}_{\mathcal{E}}: \overline{W} \rightarrow V$, has the following form:
\begin{equation*}
(\overline{\mathcal{D}}^{\star}_{\mathcal{E}}
\overline{w})|_{e}= -\frac{1}{\mathrm{len}(e)}\sum\limits_{l \in B_{1}(e)}
\overline{w}_l \mathrm{sgn}(e,\tau_l)  \mathrm{len}(l), \ \ \forall e.
\end{equation*}
\end{lemma}

\begin{proof}
By the definition of the adjoint operator, we have
\begin{equation} \label{1-formAdjointEquation}
  \langle \overline{\mathcal{D}}_{\mathcal{E}} v, \overline w \rangle_{\overline W}
  = \langle v, -\overline{\mathcal{D}}^{\star}_{\mathcal{E}} \overline w \rangle_{V}.
\end{equation}
Using the inner products \eqref{eq:1-formInner} and \eqref{EdgeInner} in $\overline{W}$ and $V$, \eqref{1-formAdjointEquation} can be rewritten as
\begin{equation} \label{1-formInnerAdjointEquation}
  \sum\limits_{l} (\overline{\mathcal{D}}_{\mathcal{E}} v)|_l \overline w_l \mathrm{len}(l)
  = \sum\limits_{e}{ v_{e} (-\overline{\mathcal{D}}^{\star}_{\mathcal{E}} \overline w) |_{e} \mathrm{len}(e)}.
\end{equation}
Using \eqref{eq:1-formOperator}, the left-hand side of \eqref{1-formInnerAdjointEquation} is actually
\begin{equation*}
\begin{aligned}
  & \sum\limits_{l} (\overline{\mathcal{D}}_{\mathcal{E}} v)|_l \overline w_l \mathrm{len}(l) \\
  = & \sum\limits_{l}   [v]_{l} \overline w_l \mathrm{len}(l) \\
  = & \sum\limits_{l}   \Big( v_{e^+}\mathrm{sgn}(e^+,\tau_l)+v_{e^-}\mathrm{sgn}(e^-,\tau_l) \Big) \overline w_l \mathrm{len}(l) \\
  = & \sum\limits_{e} v_{e}\sum\limits_{l \in B_{1}(e)}\mathrm{sgn}(e,\tau_l) \overline w_l \mathrm{len}(l)
\end{aligned}
\end{equation*}
Therefore, we have
\begin{equation*}
  \sum\limits_{e} v_{e}\sum\limits_{l \in B_{1}(e)}\mathrm{sgn}(e,\tau_l) \overline w_l \mathrm{len}(l)
  = \sum\limits_{e}{ v_{e} (-\overline{\mathcal{D}}^{\star}_{\mathcal{E}} \overline w) |_{e} \mathrm{len}(e)}.
\end{equation*}
The assertion follows immediately.
\end{proof}

\begin{lemma} \label{lemma2}
The adjoint operator of $\widetilde{\mathcal{D}}_\mathcal{E}$, that is
$\widetilde{\mathcal{D}}^{\star}_{\mathcal{E}}: \widetilde{W} \rightarrow V$ has the following form:
\begin{equation*}
  (\widetilde{\mathcal{D}}^{\star}_{\mathcal{E}} \widetilde{w})|_{e}
  = -\frac{1}{\mathrm{len}(e)}\sum\limits_{c \in B_{2}(e)} \widetilde{w}_c \mathrm{sgn}(e,\tau_c)  \mathrm{len}(c), \ \ \forall e.
\end{equation*}
%where $B_{2}(e)$ is the set of curves associated with the edge $e$ (see Fig. \ref{fig:joint-2-formOperator}),
%and $\tau_c$ is the triangle satisfying both $e \prec \tau_c$ and $\tau_c \in \{\tau^+, \tau^-\}$.
\end{lemma}

\begin{proof}
By the definition, we have
\begin{equation} \label{2-formAdjointEquation}
  \langle \widetilde{\mathcal{D}}_{\mathcal{E}} v, \widetilde w \rangle_{\widetilde W}
  = \langle v, -\widetilde{\mathcal{D}}^{\star}_{\mathcal{E}} \widetilde w \rangle_{V}.
\end{equation}
Using the inner products \eqref{eq:2-formInner} and \eqref{EdgeInner} in $\widetilde{W}$ and $V$, \eqref{2-formAdjointEquation} can be rewritten as
\begin{equation} \label{2-formInnerAdjointEquation}
  \sum\limits_{c} (\widetilde{\mathcal{D}}_{\mathcal{E}} v)|_c \widetilde{w}_c \mathrm{len}(c)
  = \sum\limits_{e}{ v_{e} (-\widetilde{\mathcal{D}}^{\star}_{\mathcal{E}} \widetilde w) |_{e} \mathrm{len}(e)}.
\end{equation}
Using \eqref{eq:2-formOperator}, the left-hand side of \eqref{2-formInnerAdjointEquation} is actually
\begin{equation*}
\begin{aligned}
  & \sum\limits_{c} (\widetilde{\mathcal{D}}_{\mathcal{E}} v)|_c \widetilde{w}_c \mathrm{len}(c) \\
  = & \sum\limits_{c} [[v]]_c \widetilde{w}_c \mathrm{len}(c) \\
  = & \sum\limits_{c} \Big( v_{e^{--}}\mathrm{sgn}(e^{--},\tau^-) + v_{e^+}\mathrm{sgn}(e^+,\tau^+) \\
  & + v_{e^-}\mathrm{sgn}(e^-,\tau^-) + v_{e^{++}}\mathrm{sgn}(e^{++},\tau^+) \Big) \widetilde{w}_c \mathrm{len}(c) \\
  = & \sum\limits_{e} v_{e}\sum\limits_{c \in B_2(e)}\mathrm{sgn}(e,\tau_c) \widetilde w_c \mathrm{len}(c).
\end{aligned}
\end{equation*}
Therefore, we have
\begin{equation*}
  \sum\limits_{e} v_{e}\sum\limits_{c \in B_2(e)}\mathrm{sgn}(e,\tau_c) \widetilde w_c \mathrm{len}(c)
   = \sum\limits_{e}{ v_{e} (-\widetilde{\mathcal{D}}^{\star}_{\mathcal{E}} \widetilde w) |_{e} \mathrm{len}(e)}.
\end{equation*}
The assertion follows immediately.
\end{proof}
